# Supplementary material for: Preference-Based Batch and Sequential Teaching: Towards a Unified View of Models
Source: arXiv:1910.10944 source file (2019-10-24)
Supplement: Supplementary file 1 [file 7.4.5_appendix_seq-models_linearVCD_examples-appendixA.tex]

% !TEX root =  main.tex
%%%%%%%%%%%%%%%%%%%%%%%%%%%%%%%%%%%%%%%%%%%%%%%%%%%%%%%%%%
%%%%%%%%%%%%%%%%%%%%%%%%%%%%%%%%%%%%%%%%%%%%%%%%%%%%%%%%%%
\clearpage
\subsection{Example of $\SigmaLvs$: Hypothesis Class in \tableref{tab:batch_model_example_h2} %~\ref{sec.appendix.batch_models.example}
}
\todo{Mention that we get TD-sigma=2.. but we can also get 1.. gvs=1}
Consider hypothesis class specified in \tableref{tab:h2} of Appendix~\ref{sec.appendix.batch_models.example}. In \tableref{tab:batch-example-lvs-proof} we have represented the preference function $\sigma_{\lvs} \in \SigmaLvs$ and teaching sequence $\Teacher_{\lvs}$ constructed in proof of \thmref{thm:main:seq-models_vs_VCD}. Here, the starting hypothesis is $\hypothesis_1$.
%, and global numbering $g(.)$ on hypotheses space which we introduced in our proof is in order of hypotheses shown in \tableref{tab:h2}. 
Also, we have chosen $\{\instance_2, \instance_3, \instance_4, \instance_5\}$ as the starting compact distinguishable set on $\Hypotheses$ (there are other alternatives). Now, \figref{fig:batch-example-lvs-proof} is showing how the learner moves along hypotheses when she receives teaching examples.

\begin{figure}[h!]
    \centering
    \includegraphics[width = 0.6\linewidth]{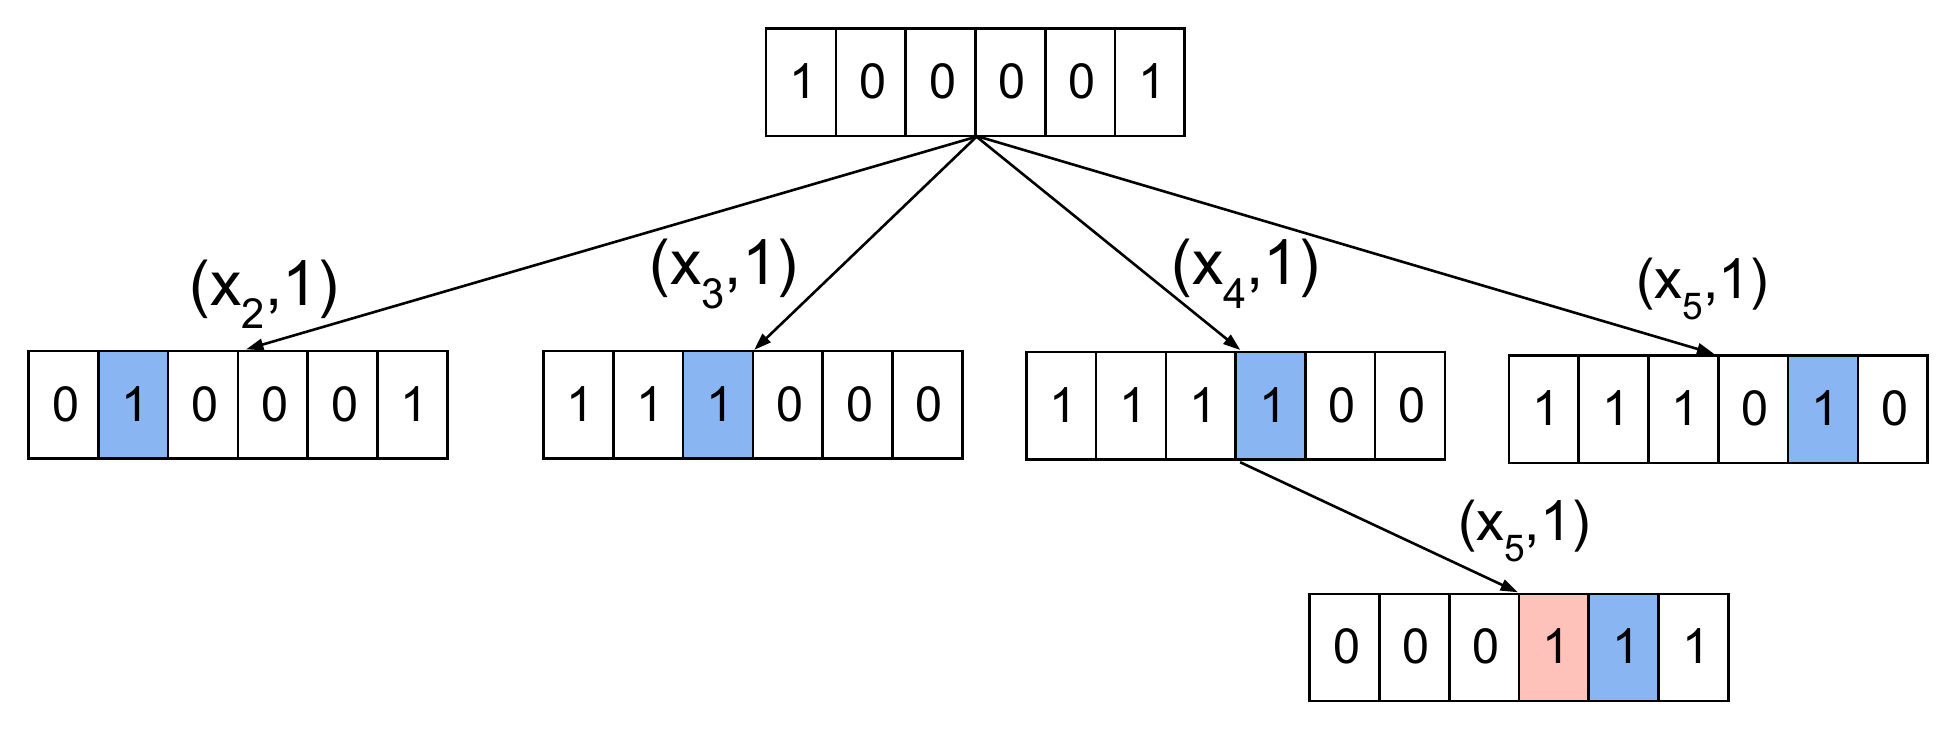}
    \caption{Graph representation of proof of Theorem~\ref{thm:main:seq-models_vs_VCD} for Table~\ref{tab:h2} in Appendix~\ref{sec.appendix.batch_models.example}.}
    \label{fig:batch-example-lvs-proof}
\end{figure}

\begin{table}[h!]
\hspace{0.1\linewidth}
\begin{subtable}[t]{0.45\textwidth}
\centering
\scalebox{0.9}{
\begin{tabular}{c|c|c|c}
\textbf{$\hypotheses$} & $\hypothesis$ & $\hypothesis'$ & $\sigma_{lvs}$ \\ \hline
\multirow{2}{*}{$\{\hypothesis_2, \hypothesis_3, \hypothesis_4, \hypothesis_5\}$} & \multirow{2}{*}{$\hypothesis_1$} & $\hypothesis_2$ & 2 \\
 &  & others & 7 \\\hline
\multirow{2}{*}{$\{\hypothesis_3, \hypothesis_4, \hypothesis_5\}$} & \multirow{2}{*}{$\hypothesis_1$} & $\hypothesis_3$ & 3 \\
  &  & others & 7 \\\hline
\multirow{3}{*}{$\{\hypothesis_4, \hypothesis_6\}$} & \multirow{3}{*}{$\hypothesis_1$} & $\hypothesis_4$ & 4 \\
 &  & $\hypothesis_6$ & 6 \\
 &  & others & 7 \\\hline
 \multirow{2}{*}{$\{\hypothesis_5, \hypothesis_6\}$} & \multirow{2}{*}{$\hypothesis_1$} & $\hypothesis_5$ & 5 \\
  &  & others & 7 \\\hline
  
\multirow{2}{*}{$\{\hypothesis_6\}$} & \multirow{2}{*}{$\hypothesis_4$} & $\hypothesis_6$ & 6 \\
  &  & others & 7 \\\hline

\end{tabular}}
\caption{The preference function $\sigma_{lvs}$. For all other $\hypothesis', \hypotheses, \hypothesis$ tuples not specified in the table, $\sigma(\hypothesis'; \hypotheses, \hypothesis) = 8$ if $\hypothesis' \neq \hypothesis$, and $\sigma(\hypothesis'; \hypotheses, \hypothesis) = 0$ if $\hypothesis' = \hypothesis$.}\label{tab:batch-example-lvs-pref-proof}
\end{subtable}
\quad
\begin{subtable}[t]{0.4\textwidth}
\centering
\scalebox{0.9}{
\begin{tabular}{c|c}
hypothesis & $\Teacher_{\lvs}$ \\ \hline
$\hypothesis_1$ & $\{(\instance_2, 0)\}$ \\
$\hypothesis_2$ & $\{(\instance_2, 1)\}$ \\
$\hypothesis_3$ & $\{(\instance_3, 1)\}$ \\
$\hypothesis_4$ & $\{(\instance_4, 1)\}$ \\
$\hypothesis_5$ & $\{(\instance_5, 1)\}$ \\
$\hypothesis_6$ & $\{(\instance_4, 1), (\instance_5, 1)\}$ \\
\end{tabular}}\caption{Teaching sequence for all hypotheses.}\label{tab:batch-example-lvs-teach-seq-proof}
\end{subtable}
\caption{Preference Function and teaching sequence constructed in proof of \thmref{thm:main:seq-models_vs_VCD} for \tableref{tab:h2} in Appendix~\ref{sec.appendix.batch_models.example}.}\label{tab:batch-example-lvs-proof}
\end{table}
