# Supplementary material for: Preference-Based Batch and Sequential Teaching: Towards a Unified View of Models
Source: arXiv:1910.10944 source file (2019-10-24)
Supplement: Supplementary file 2 [file 7.5_appendix_rebuttal-proof-tdsigma-is-not-constant.tex]

% !TEX root =  main.tex
%%%%%%%%%%%%%%%%%%%%%%%%%%%%%%%%%%%%%%%%%%%%%%%%%%%%%%%%%%
%%%%%%%%%%%%%%%%%%%%%%%%%%%%%%%%%%%%%%%%%%%%%%%%%%%%%%%%%%
%\clearpage
\section{$\Sigmatd{}$ is not constant}
%\todo{Cleanup if we want to keep this proof}
Based on definition of teaching sequence, for any two hypotheses teaching sequence cannot be exactly the same (They can be with different orders). Now, Assume that $\Hypotheses$, $\Instances$ are representing power set of size $d$. We know that $|\Instances| = d$, $|\Hypotheses| = 2^d$, and $\VCD(\Hypotheses) = d$. Also consider $k = \Sigmatd{\Instances, \Hypotheses, \hypothesis_0}$. We'll denote $N(k)$ to be number of teaching sequence of size less than or equal to $k$. Notice that the total number of unique teaching sequences of size less than or equal to $k$ must be greater than or equal to $|\Hypotheses|$, i.e., $N(k) \geq |\Hypotheses|$.  Furthermore, since $d \geq 1$, we have that
\begin{equation*}
    N(k) \leq \sum_{i = 0}^k (2|\Instances|)^i = \sum_{i = 0}^k (2d)^i < (2d)^{k+1}.
\end{equation*}
We will conclude that $2^d < (2d)^{k+1}$. This indicates that $k$ is $\Omega\big({\frac{d}{\log d}}\big)$.
 
