# Supplementary material for: Preference-Based Batch and Sequential Teaching: Towards a Unified View of Models
Source: arXiv:1910.10944 source file (2019-10-24)
Supplement: Supplementary file 3 [file 8_appendix_farnam-rebuttal-problems.tex]

% !TEX root =  main.tex
%%%%%%%%%%%%%%%%%%%%%%%%%%%%%%%%%%%%%%%%%%%%%%%%%%%%%%%%%%
%%%%%%%%%%%%%%%%%%%%%%%%%%%%%%%%%%%%%%%%%%%%%%%%%%%%%%%%%%
\clearpage
\section{Farnam Mansouri -- Rebuttal technical problems}

\subsection{is $TD(\Instances, \Hypotheses, \hypothesis_0)$ sub-additive or additive?}
\subsubsection{definition}
First we will formally define additive and sub-additive based on \cite{DBLP:journals/jmlr/DoliwaFSZ14}. Consider two hypothesis space $\Hypotheses_1$ and $\Hypotheses_2$, over two disjoint instances space respectively $\Instances_1$ and $\Instances_2$, i.e.,  $\Instances_1 \cap \Instances_2 = \varnothing$. We'll define $\Hypotheses_1 \uplus \Hypotheses_2 = \{A \cup B | A \in \Hypotheses_1, B \in \Hypotheses_2\}$.


We denote a family of preference functions $\Sigma$ additive over $\uplus$, if $\forall \Hypotheses_1, \Hypotheses_2,  \Instances_1, \Instances_2, \hypothesis_0^1 \in \Hypotheses_1,  \hypothesis_0^2 \in \Hypotheses_2: \Sigmatd{\Instances_1 \cup \Instances_2, \Hypotheses_1 \uplus \Hypotheses_2, \hypothesis_0^1 \cup \hypothesis_0^2} = \Sigmatd{\Instances_1, \Hypotheses_1,\hypothesis_0^1} + \Sigmatd{\Instances_2, \Hypotheses_2,\hypothesis_0^2}$.


\subsubsection{$\Sigmatd{}$ is sub-additive for families with a property}
Consider $\Hypotheses_1$, $\Instances_1$, $\hypothesis^1_0 \in \Hypotheses_1$, and $\Hypotheses_2$, $\Instances_2$, $\hypothesis^2_0 \in \Hypotheses_2$. Let $\sigma_1 \in \argmin_\sigma \TD(\Instances_1, \Hypotheses_1, \sigma, \hypothesis^1_0)$, $\sigma_2 \in \argmin_\sigma \TD(\Instances_2, \Hypotheses_2, \sigma, \hypothesis^2_0)$ be the best preference functions.

% If for some $\hypotheses \subseteq \Hypotheses_1$ and $\hypothesis, \hypothesis', \hypothesis'' \in \hypotheses$ we have that $\sigma_1(\hypothesis'; \hypothesis, \hypotheses) = \sigma_1(\hypothesis''; \hypothesis, \hypotheses)$ we can simply assume that $\sigma_1(\hypothesis'; \hypothesis, \hypotheses) > \sigma_1(\hypothesis''; \hypothesis, \hypotheses)$. Considering the definition of $\TD(\Instances_1, \Hypotheses_1, \sigma_1, \hypothesis^1_0)$, $\TD(\Instances_1, \Hypotheses_1, \sigma_1, \hypothesis^1_0)$ wouldn't decrease, and if $\Sigma$ isn't $\Sigma-const$, we can still have $\sigma_1 \in \Sigma$. This indicates that there is always an optimal $\sigma_1$, where $\hypothesis'$ has a strict order if we fix other domains. Also, we can argue the same for 

In this section we want to prove that for a restricted family preference functions, which have following property. If current hypothesis $\hypothesis$ is in next version space $V$. Then $\hypothesis$ should minimize $\sigma(.; \hypothesis, V)$.



For $\sigma_1, \sigma_2 \in \Sigma$, we'll define $\sigma = \sigma_1 \uplus \sigma_2$ over hypotheses space $\Hypotheses_1 \uplus \Hypotheses_2$ as follows. For any hypothesis $\hypothesis_1, \hypothesis'_1 \in \Hypotheses_1$, $\hypothesis_2, \hypothesis'_2 \in \Hypotheses_2$, and version space $V_1 \subseteq \Hypotheses_1$, $V_2\subseteq \Hypotheses_2$, we'll denote $\sigma(\hypothesis'_1 \cup \hypothesis'_2; \hypothesis_1 \cup \hypothesis_2; V_1 \uplus V_2) := M * \sigma_1(\hypothesis'_1; \hypothesis_1; V_1) + \sigma_2(\hypothesis'_2; \hypothesis_2; V_2)$, where $M > \max_{h_1, h'_1, h_2, h'_2, V_1, V_2}{|\sigma_2|/|\sigma_1|}$ is a large number.


Let the starting hypothesis in $\Hypotheses_1 \uplus \Hypotheses_2$ be $\hypothesis^1_0 \cup \hypothesis^2_0$. Also, the target hypothesis $\hypothesis^*_1 \cup \hypothesis^*_2$. If we provide instances from $\Instances_2$, the version space left would always be $\Hypotheses_1 \uplus V_2$, where $V_2$ is version space after teaching same examples from $\Instances_2$. Now, $\sigma(\hypothesis'_1 \cup \hypothesis'_2; \hypothesis^1_0 \cup \hypothesis_2; \Hypotheses_1 \uplus V_2) := M \sigma_1(\hypothesis'_1; \hypothesis^1_0,  \Hypotheses_1) + \sigma_2(\hypothesis'_2; \hypothesis_2, V_2)$. First part of $\sigma$ will always be $\sigma_1(. ; \hypothesis^1_0, \Hypotheses_1)$. As we have assumed in this family of preference functions $\sigma_1(. ; \hypothesis^1_0, \Hypotheses_1)$ will be maximized in $\sigma_1(. ; \hypothesis^1_0, \Hypotheses_1)$.


Therefore, it is easy to see with $\TD(\Instances_2, \Hypotheses_2, \sigma_2, \hypothesis^2_0)$ teaching examples, learner can reach $\hypothesis^1_0 \cup \hypothesis^*_2$. Furthermore, with similar arguments, learner can reach $\hypothesis^*_1 \cup \hypothesis^*_2$ from $\hypothesis_1^0 \cup \hypothesis^*_2$ with $\TD(\Instances_1, \Hypotheses_2, \sigma_2, \hypothesis^2_0)$. We will conclude that $\Sigmatd{\Instances_1 \cup \Instances_2, \Hypotheses_1 \uplus \Hypotheses_2, \hypothesis_0^1 \cup \hypothesis_0^2} \leq \Sigmatd{\Instances_1, \Hypotheses_1,\hypothesis_0^1} + \Sigmatd{\Instances_2, \Hypotheses_2,\hypothesis_0^2}$.

\begin{corollary}
Here we are going to have another statement for normal families. We can simply reach from $\hypothesis^1_0 \cup \hypothesis^2_0$ to some $\hypothesis_i \cup \hypothesis^*_2$ for some $i$ , if teacher gives the teaching set for $\Hypotheses_2$ (because independant of first part of $\sigma$ teacher can optimize second part, and first end up in some place). And since teaching is collision free if teacher provides more examples from $\Instances_2$ the second part will be minimized at $\hypothesis^*_2$. This indicates that $\TD(\Instances_1 \cup \Instances_2, \Hypotheses_1 \uplus \Hypotheses_2, \sigma_1 \uplus \sigma_2, \hypothesis^1_0 \cup \hypothesis^2_0) \leq \TD(\Instances_1, \Hypotheses_1, \sigma_1, \hypothesis_i) + \TD(\Instances_2, \Hypotheses_2, \sigma_2, \hypothesis^2_0)$. We can conclude that $\max_{\hypothesis \in \Hypotheses_1 \uplus \Hypotheses_2} \Sigmatd{\Instances_1 \cup \Instances_2, \Hypotheses_1 \uplus \Hypotheses_2, \hypothesis} \leq \max_{\hypothesis \in \Hypotheses_1} \Sigmatd{\Instances_1, \Hypotheses_1, \hypothesis} + \max_{\hypothesis \in \Hypotheses_2} \Sigmatd{\Instances_2, \Hypotheses_2, \hypothesis}$.
\end{corollary}

\subsection{$\Sigmatd{}$ is not constant}
Based on definition of teaching sequence, for any two hypotheses teaching sequence cannot be exactly the same (They can be with different orders). Now, Assume that $\Hypotheses$, $\Instances$ are representing power set of size $d$. We know that $|\Instances| = d$, $|\Hypotheses| = 2^d$, and $\VCD(\Hypotheses) = d$. Also consider $k = \Sigmatd{\Instances, \Hypotheses, \hypothesis_0}$. We'll denote $N(k)$ to be number of teaching sequence of size less than or equal to $k$. Notice that the total number of unique teaching sequences of size less than or equal to $k$ must be greater than or equal to $|\Hypotheses|$, i.e., $N(k) \geq |\Hypotheses|$.  Furthermore, since $d \geq 1$, we have that
\begin{equation*}
    N(k) \leq \sum_{i = 0}^k (2|\Instances|)^i = \sum_{i = 0}^k (2d)^i < (2d)^{k+1}.
\end{equation*}
We will conclude that $2^d < (2d)^{k+1}$. This indicates that $k$ is $\Omega\big({\frac{d}{\log d}}\big)$.
 
\subsection{Infinite domain.}
Well, we can say that $\Sigmatd{global} := \PBTD$ (In paper we have RTD which are equal only in finite domain). But our main result cannot be generalized to infinite domain, because we are enumerating the instances space for creating the partitions in lemma 4.Enumerating instance space is only possible when instance space size is countable. For example consider $\Hypotheses$ to be all linear classifiers on instance space $\Instances = R^2$, non two hypotheses are different on only one example. This indicates that, $\forall \clabel \in \{0, 1\}, \instance \in \Instances: \Hypotheses^\clabel_\instance = \varnothing$. In other words, our algorithm doesn't work for this hypotheses space. Finding an algorithm which also works for uncountable instance space domain can be an open problem for future work.

\subsection{Theorem 9 of Sample compression, learnability and the Vapnik-Chervonenkis dimension}
The similarity is that $C^{\{x\}}$ is equal to our definition of $C^0_x$. They used the induction on $C^{\{x\}}$, and $C - x$. These two are represented respectively as $C^0_x$, and $C \setminus C^0_x$ in our paper. In principle, they have partitioned $C$ to $n$, $d - 1$ VC dimension group.
